# Supplementary material for: TedNet: A Pytorch Toolkit for Tensor Decomposition Networks
Source: arXiv:2104.05018 source file (2021-11-21)
Supplement: Supplementary file 1 [file appendix.tex]

\newpage

\appendix
\section*{Appendix A.}
\label{app:theorem}

% Note: in this sample, the section number is hard-coded in. Following
% proper LaTeX conventions, it should properly be coded as a reference:

%In this appendix we prove the following theorem from
%Section~\ref{sec:textree-generalization}:

In this appendix we prove the following theorem from
Section~6.2:

\noindent
{\bf Theorem} {\it Let $u,v,w$ be discrete variables such that $v, w$ do
not co-occur with $u$ (i.e., $u\neq0\;\Rightarrow \;v=w=0$ in a given
dataset $\dataset$). Let $N_{v0},N_{w0}$ be the number of data points for
which $v=0, w=0$ respectively, and let $I_{uv},I_{uw}$ be the
respective empirical mutual information values based on the sample
$\dataset$. Then
\[
	N_{v0} \;>\; N_{w0}\;\;\Rightarrow\;\;I_{uv} \;\leq\;I_{uw}
\]
with equality only if $u$ is identically 0.} \hfill\BlackBox

\noindent
{\bf Proof}. We use the notation:
\[
P_v(i) \;=\;\frac{N_v^i}{N},\;\;\;i \neq 0;\;\;\;
P_{v0}\;\equiv\;P_v(0)\; = \;1 - \sum_{i\neq 0}P_v(i).
\]
These values represent the (empirical) probabilities of $v$
taking value $i\neq 0$ and 0 respectively.  Entropies will be denoted
by $H$. We aim to show that $\fracpartial{I_{uv}}{P_{v0}} < 0$....\\
